# Supplementary material for: Multi-Instance Pose Networks: Rethinking Top-Down Pose Estimation
Source: arXiv:2101.11223 source file (2021-10-28)
Supplement: Supplementary file 2 [file block_placement.tex]

\begin{table}
\centering
 % Default value: 1
    \begin{tabular}{@{}c|c c c|c c c @{}}
    \hline
    MIMBs & \multicolumn{3}{c|}{COCO} & \multicolumn{3}{c}{OCHuman}\\
    Placement & $\text{AP}$ & $\text{AP}^{50}$ & $\text{AP}^{75}$ & $\text{AP}$ & $\text{AP}^{50}$ & $\text{AP}^{75}$  \\
    \hline
    Stage 1 & 78.7 & 94.4 & 85.4 & 72.3 & 89.7 & 78.2 \\
    Stage 2 & 78.8 & 94.4 & 85.6 & 74.0 & 90.1 & 80.3\\
    Stage 3 & 78.8 & 94.4 & 85.8 & 74.4 & 90.7 & 80.9\\
    Stage 4 & 78.5 & 94.4 & 85.5 & 70.8 & 89.8 & 77.5\\
    \hline
    %Arch & Placement & AP & AP $.5$ & AP $.75$ & AP(M) & AP(L) & AR & AR $.5$ & AR $.75$ & AR (M) & AR (L) \\

    % & & \multicolumn{9}{c}{COCO} & \\

    % Stage 1 & 78.5 & 94.4 & 85.5 & 75.3 & 83.5 & 81.4 & 95.8 & 87.5 & 77.8 & 86.7 \\
    % $[0, 0, 1, 0]$ & 78.8 & 94.4 & 85.8 & 75.5 & 83.6 & 81.5 & 95.4 & 87.8 & 78.0 & 86.6 \\
    % $[0, 1, 0, 0]$ & 78.8 & 94.4 & 85.6 & 75.8 & 83.6 & 81.7 & 95.7 & 87.7 & 78.3 & 86.8 \\
    % Stage 1 & & & & & & & & & & \\
    % & & \multicolumn{9}{c}{OCHuman} & \\
    % $[0, 0, 0, 1]$ & 70.8 & 89.8 & 77.5 & 65.7 & 70.9 & 77.9 & 94.2 & 84.2 & 68.6 & 77.9 \\
    % MHPNet-W48 & $[0, 0, 1, 0]$ & 74.4 & 90.7 & 80.9 & 66.9 & 74.4 & 81.2 & 95.1 & 87.2 & 70.0 & 81.2 \\
    % MHPNet-W48 & $[0, 1, 0, 0]$ & 74.0 & 90.1 & 80.3 & 63.6 & 74.0 & 80.7 & 94.5 & 86.7 & 68.6 & 80.7 \\
    % MHPNet-W48 & $[1, 0, 0, 0]$ & & & & & & & & & & \\

    \end{tabular}
    \caption{MIMBs placement at various stages in HRNet and its impact on COCO and OCHuman \texttt{val} sets using ground truth bounding boxes.}
    \label{tab:block_placement}
\end{table}
